# Supplementary material for: Controllable Capillary Assembly of Magnetic Ellipsoidal Janus Particles into Tunable Rings, Chains and Hexagonal Lattices
Source: arXiv:2009.09804 ancillary file (2020-12-27)
Supplement: Supplementary file 1 [file main-supp-arxiv.pdf]

# Supplementary Material For "Controllable Capillary Assembly of Magnetic Ellipsoidal Janus Particles into Tunable Rings, Chains and Hexagonal Lattices"

Qingguang Xie<sup>1</sup> and Jens Harting<sup>2,3,\*</sup>

<sup>1</sup>*Department of Applied Physics, Eindhoven University of Technology,  
P.O. Box 513, 5600MB Eindhoven, The Netherlands*

<sup>2</sup>*Helmholtz Institute Erlangen-Nürnberg for Renewable Energy (IEK-11),  
Forschungszentrum Jülich, Fürther Str. 248, 90429 Nürnberg, Germany*

<sup>3</sup>*Department of Chemical and Biological Engineering and Department of Physics,  
Friedrich-Alexander-Universität Erlangen-Nürnberg,  
Fürther Straße 248, 90429 Nürnberg, Germany*

---

\* j.harting@fz-juelich.de

## I. SIMULATION METHOD

We use the lattice Boltzmann method (LBM) to simulate the motion of each fluid. The LBM is a local mesoscopic algorithm, allowing for efficient parallel implementation, and has demonstrated itself as a powerful tool for numerical simulations of fluid flows. [1] It has been extended to allow the simulation of, for example, multiphase/multicomponent fluids [2–4] and suspensions of particles of arbitrary shape and wettability. [5–8]

We implement the pseudopotential multicomponent LBM method of Shan and Chen [2] with a D3Q19 lattice [9] and review some relevant details in the following. Two fluid components follow the Boltzmann equation discretized in space and time,

$$f_i^c(\vec{x} + \vec{c}_i \Delta t, t + \Delta t) = f_i^c(\vec{x}, t) + \Omega_i^c(\vec{x}, t), \quad (1)$$

where  $i = 1, \dots, 19$ ,  $f_i^c(\vec{x}, t)$  are the single-particle distribution functions for fluid component  $c = 1$  or  $2$ ,  $\vec{c}_i$  is the discrete velocity in the  $i$ th direction, and

$$\Omega_i^c(\vec{x}, t) = -\frac{f_i^c(\vec{x}, t) - f_i^{\text{eq}}(\rho^c(\vec{x}, t), \vec{u}^c(\vec{x}, t))}{(\tau^c / \Delta t)} \quad (2)$$

is the Bhatnagar-Gross-Krook (BGK) collision operator. [10]  $\tau^c$  is the relaxation time for component  $c$ . The macroscopic densities and velocities are defined as  $\rho^c(\vec{x}, t) = \rho_0 \sum_i f_i^c(\vec{x}, t)$ , where  $\rho_0$  is a reference density, and  $\vec{u}^c(\vec{x}, t) = \sum_i f_i^c(\vec{x}, t) \vec{c}_i / \rho^c(\vec{x}, t)$ , respectively. Here,  $f_i^{\text{eq}}(\rho^c(\vec{x}, t), \vec{u}^c(\vec{x}, t))$  is a second-order equilibrium distribution function. [11] When sufficient lattice symmetry is guaranteed, the Navier-Stokes equations can be recovered from Eq. (1) on appropriate length and time scales [1]. For convenience we choose the lattice constant  $\Delta x$ , the timestep  $\Delta t$ , the unit mass  $\rho_0$  and the relaxation time  $\tau^c$  to be unity, which leads to a kinematic viscosity  $\nu^c = \frac{1}{6}$  in lattice units.

For fluids to interact, we introduce a mean-field interaction force between fluid components  $c$  and  $c'$  following a pseudopotential approach. [2] The pseudopotential LBM of Shan and Chen is a diffuse interface method, resulting in an interface width of  $\approx 5\Delta x$ . The particle is discretized on the fluid lattice and coupled to the fluid species by means of a modified bounce-back boundary condition as pioneered by Ladd and Aidun. [5, 6]. For a detailed description of the method including the extension to particles suspended in multicomponent flows, we refer the reader to the relevant literature. [7, 8, 12–16]

We perform simulations with a system of size  $256 \times 128 \times 256$ . For single Janus particles, we fix the radii to  $a = 10$ ,  $c = 30$ . For multiple Janus particles, we reduce the radii to

$a = 6, c = 18$ . The upper half of the system is filled with fluid 1 and the lower one with fluid 2 leading to a well defined interface in the center of the system. Additionally, we impose walls with mid-grid bounce back boundary conditions at the top and bottom of the system parallel to the interface, while all other boundaries are periodic.

## II. SUPPLEMENTARY SIMULATION RESULTS

Supplementary Movie S1 shows the structural transitions when the external magnetic fields are varied.

Fig. S1 shows the interface deformation around a single ellipsoidal Janus particle with aspect ratio  $\alpha = 3$  and amphiphilicity  $\beta = 21^\circ$  at different tilt angles.

Fig. S2 shows the interface deformation around a single ellipsoidal Janus particle with aspect ratio  $\alpha = 3$  and amphiphilicities  $\beta = 39^\circ$  at tilt angle  $\varphi = 75^\circ$  and  $\varphi = 85^\circ$ .

Fig. S3 shows the alignment of two ellipsoidal Janus particles with aspect ratio  $\alpha = 3$  and amphiphilicity  $\beta = 21^\circ$  without and with external magnetic fields.

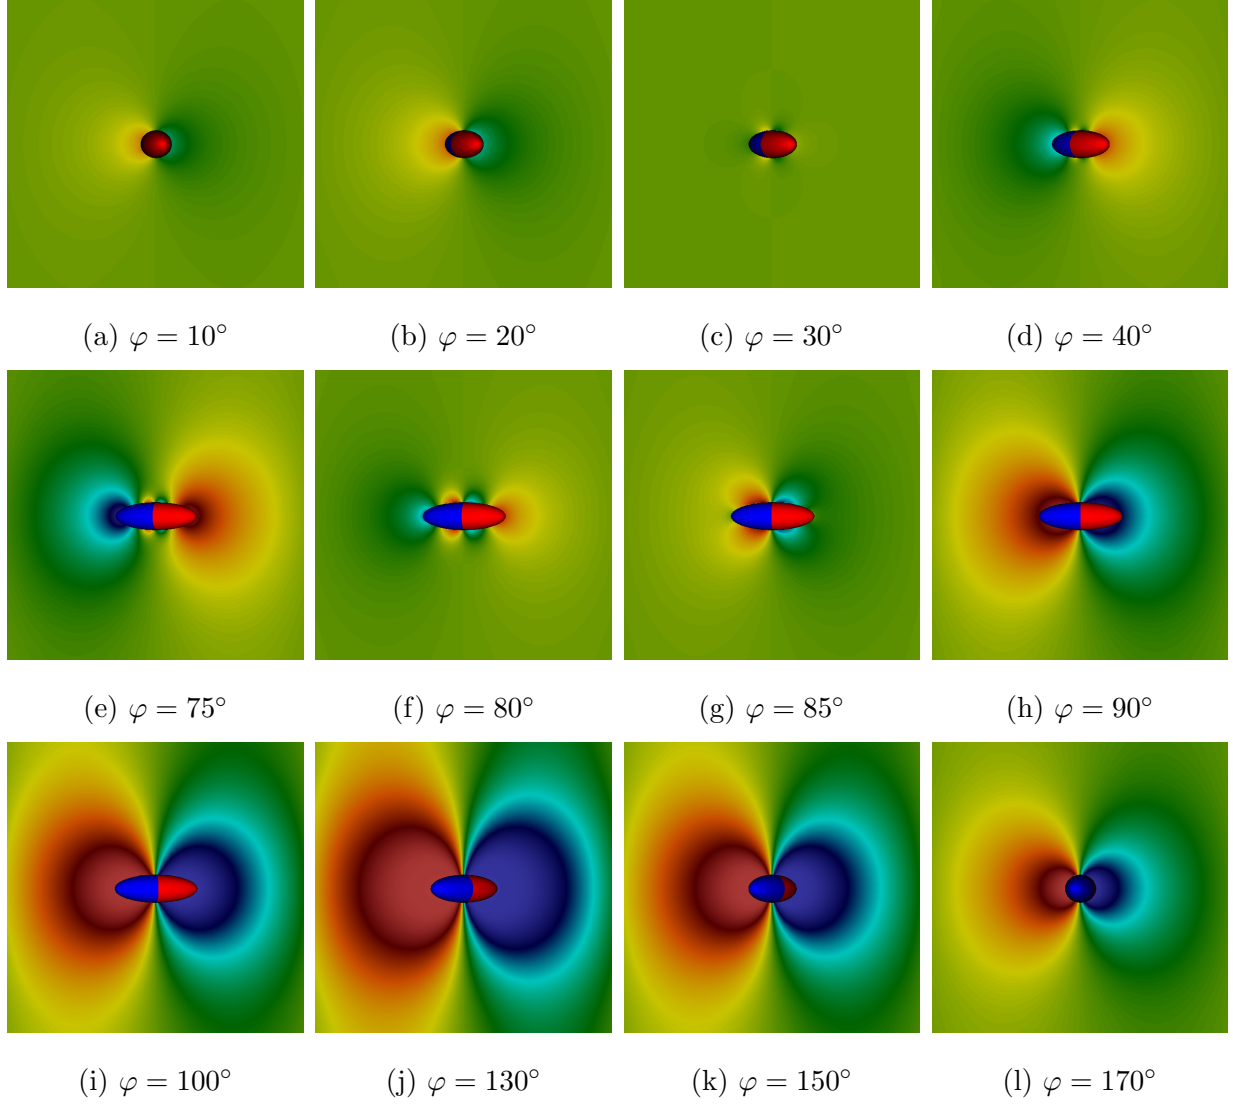

FIG. S1: Interface deformation around a single ellipsoidal Janus particle with aspect ratio  $\alpha = 3$  and amphiphilicity  $\beta = 21^\circ$  at different tilt angles.

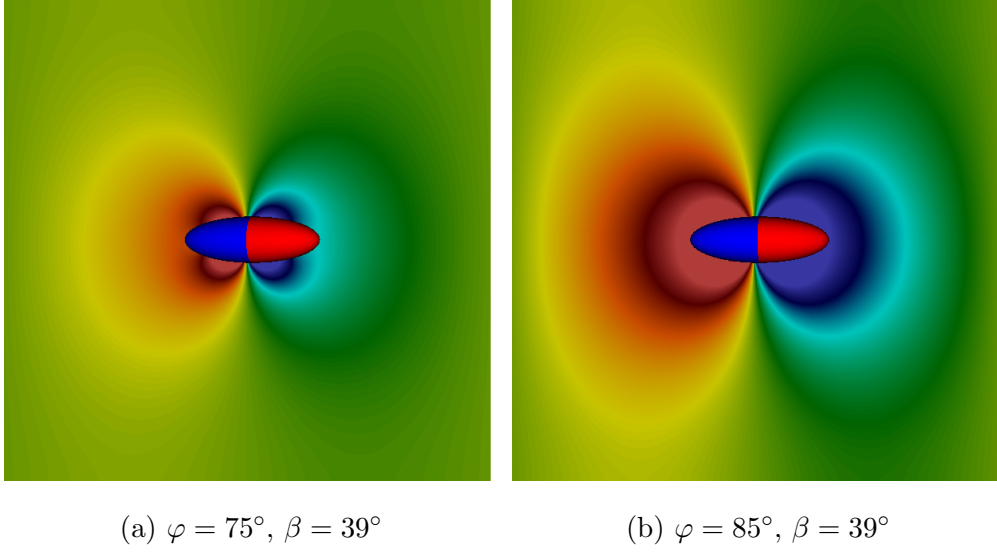

FIG. S2: Interface deformation around a single ellipsoidal Janus particle with aspect ratio  $\alpha = 3$  and amphiphilicities  $\beta = 39^\circ$  at tilt angle  $\varphi = 75^\circ$  and  $\varphi = 85^\circ$ . The particle generates a unsymmetrical hexapolar interface deformation a) and dipolar deformation b).

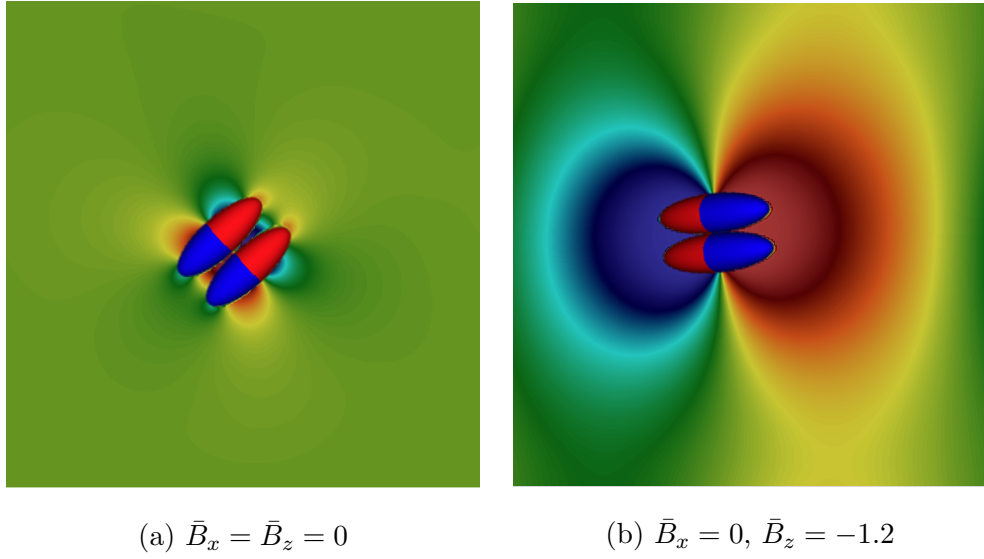

FIG. S3: Alignment of two ellipsoidal Janus particle with aspect ratio  $\alpha = 3$  and amphiphilicity  $\beta = 21^\circ$  without a) and with b) external magnetic fields.

- 
- [1] S. Succi. *The Lattice Boltzmann Equation: For Fluid Dynamics and Beyond*. Oxford University Press, 2001.
- [2] X. Shan and H. Chen. Lattice Boltzmann model for simulating flows with multiple phases and components. *Phys. Rev. E*, 47:1815, 1993.
- [3] X. Shan and H. Chen. Simulation of nonideal gases and liquid-gas phase transitions by the lattice Boltzmann equation. *Phys. Rev. E*, 49:2941, 1994.
- [4] H. Liu, Q. Kang, C. R. Leonardi, S. Schmieschek, A. I. Narváez, B. D. Jones, J. R. Williams, A. J. Valocchi, and J. Harting. Multiphase lattice Boltzmann simulations for porous media applications. *Computat. Geosci.*, 20:777–805, 2016.
- [5] A. J. C. Ladd and R. Verberg. Lattice-Boltzmann Simulations of Particle-Fluid Suspensions. *J. Stat. Phys.*, 104:1191–1251, 2001.
- [6] C. K. Aidun, Y. Lu, and E.-J. Ding. Direct Analysis of Particulate Suspensions with Inertia Using the Discrete Boltzmann Equation. *J. Fluid Mech.*, 373:287–311, 1998.
- [7] F. Jansen and J. Harting. From bijels to Pickering emulsions: a lattice Boltzmann study. *Phys. Rev. E*, 83:046707, 2011.
- [8] F. Günther, F. Janoschek, S. Frijters, and J. Harting. Lattice Boltzmann Simulations of Anisotropic Particles at Liquid Interfaces. *Comput. Fluids*, 80:184–189, 2013.
- [9] Y. H. Qian, D. D’Humières, and P. Lallemand. Lattice BGK models for Navier-Stokes equation. *Europhys. Lett.*, 17:479–484, 1992.
- [10] P.L. Bhatnagar, E.P. Gross, and M. Krook. A model for collision processes in gases. I. Small amplitude processes in charged and neutral one-component systems. *Phys. Rev.*, 94:511–525, 1954.
- [11] H. Chen, S. Chen, and W. H. Matthaeus. Recovery of the Navier-Stokes equations using a lattice-gas Boltzmann method. *Phys. Rev. A*, 45, 1992.

- [12] A. Komnik, J. Harting, and H. J. Herrmann. Transport phenomena and structuring in shear flow of suspensions near solid walls. *Journal of Statistical Mechanics: theory and experiment*, P12003, 2004.
- [13] S. Frijters, F. Günther, and J. Harting. Effects of nanoparticles and surfactant on droplets in shear flow. *Soft Matter*, 8:6542–6556, 2012.
- [14] S. Cappelli, Q. Xie, J. Harting, A. M. de Jong, and M. W. J. Prins. Dynamic wetting: status and prospective of single particle based experiments and simulations. *New Biotechnol.*, 32:420–32, 2015.
- [15] T. Krüger, S. Frijters, F. Günther, B. Kaoui, and J. Harting. Numerical simulations of complex fluid-fluid interface dynamics. *Eur. Phys. J. Special Topics*, 222:177–198, 2013.
- [16] Q. Xie and J. Harting. From dot to ring: the role of friction on the deposition pattern of a drying colloidal suspension droplet. *Langmuir*, 34:5303–5311, 2018.
